# Supplementary material for: Learning to Play Against Unknown Opponents
Source: arXiv:2412.18297 source file (2025-02-20)
Supplement: Supplementary file 1 [file appendixOPT.tex]

\subsection{Geometric Preliminaries}
\begin{definition}[Point-to-set Distance] For some point $x$ in $\mathbb{R}^{d}$ and some convex set $D$ in $\mathbb{R}^{d}$, let the point-to-set distance $\rho(x,D) = \inf_{y \in D}||x - y||_2$.
\end{definition}

\begin{definition}[$\epsilon$-Expansion and $\epsilon$-contraction of a Set] Consider some set $D \in \mathbb{R}^{d}$. The $\epsilon$-expansion of $D$ is the set $D^{\epsilon}$ such that
\begin{equation}
    D^{\epsilon} = \{x : \rho(x,D) \leq \epsilon \}
\end{equation}

Conversely, $D$ is the $\epsilon$-contraction of $D^{\epsilon}$.
\end{definition}

\begin{definition}[The Optimizer]
    The optimizer is characterized by a public prior distribution $D$ on functions that map $\Delta^{mn} \rightarrow [-1,1]$. $D$ has support $k$, and puts probability $\alpha_i$ on payoff function $u_{O,i}$ for $i \in [k]$.
\end{definition}

The search space is over $\mathbb{R}^{mnk}$, we write points of interest, called k-CSPs in the standard form $\Phi = (\phi_1,\phi_2 \cdots \phi_k)$ where $\phi_i \in \mathbb{R}^{mn}$.

\begin{definition}[Learner Value Function]
The learner value of a candidate solution $\phi$ is $V_L(\Phi) := \sum_{i=1}^k \alpha_i u_L(\phi_i)$.
\end{definition}

\begin{definition}[Incentive Compatible Set]
The set $\cR$ (defined below) is the set of incentive compatible points:

\[ \cR := \{ \Phi \in \Delta^{mnk} | u_{O,i}(\phi_i) \ge u_{O,i}(\phi_j) \forall i,j \in [k] \}\]
    
\end{definition}

We define a canonical operation that takes any k-CSP $\Phi$ and converts it into the following polytope.

\begin{definition}[Canonical Polytope Operation]
The operation $\cC$ (defined below) converts a given k CSP set $\phi$ into a polytope contained in the $mn$-dimensional simplex :

\[ \cC(\Phi) := \{ \phi \in \Delta^{mn} | u_{O,i}(\phi) \le u_{O,i}(\phi_i) \forall i \in [k] \}\]
    
\end{definition}

\begin{definition}[Valid Menu k-CSPs]
The set $\cS$ (defined below) is the set of k-CSPs whose canonical polytope is a valid menu:

\[ \cS := \{ \Phi \in \Delta^{mnk} | \cC(\Phi) \text{ is a valid menu}.\}\]
    
\end{definition}

\begin{definition}[Feasible Set]
The feasible set of k-CSPs $\cP$ is defined to be $\cP := \cR \cap \cS$.
    
\end{definition}

Rethinking the search space in terms of k-CSPs is justified by the following lemma, which shows that an optimal commitment menu can be written as the canonical polytope operation applied on a particular k-CSP.

\begin{lemma}
    \label{lemma:succinct_opt_kcsp}
    There exists a k-CSP $\Phi^*$ such that $V_L(\Phi^*) = V_L(\cM^*)$ where $\cM^*$ is an optimal menu to commit to when playing against a prior $\cD$ of optimizers.
\end{lemma}

\begin{proof}
    Consider an optimal menu $\cM^*$. Let $\phi_1$, $\phi_2 , \cdots \phi_k$ be the CSPs ``chosen" by optimizer type $i$ in the menu $\cM^*$. Our candidate k-CSP $\Phi$ is the ordered tuple of these $k$-CSPs $\phi_1$ to $\phi_k$. Tautologically, $u_{O,i}(\phi_i) \ge u_{O,i}(\phi_j)$ for each $i,j \in [k]$, implying that $\Phi \in \cR$. To show that $\Phi \in \cS$, we show that $\cM^* \subseteq \cC(\Phi)$, since menus are upwards closed, this would complete the proof. Consider any CSP $\phi \in \cM^* \subseteq \Delta^{mn}$ and any $i \in [k]$, since the i-th optimizer weakly prefers $\phi_i$, we have $u_{O,i} (\phi_i) \ge u_{O,i}(\phi)$. Thus, this $\phi$ satisfies all the constraints required to be satisfied to be present in the polytope $\cC(\Phi)$, which finishes this proof. 
\end{proof}

Thus the original problem of this section can be rewritten as finding $\Phi \in \argmax_{\Phi \in \cP} V_L(\Phi)$.

\subsection{Convexity Proofs}

\begin{observation}
    The set $\cP$ is non-empty.
\end{observation}

\begin{proof}
    $\Phi^* = (\phi_1^*,\phi_2^*,\cdots \phi_k^*) \in \cP$ where $\phi^*_i \in \argmax_{\phi in \Delta^{mn}} u_{O,i}(\phi)$. This is because we tautologically satisfy the conditions in $\cR$ while containment in $\cS$ follows from the fact that $\cC(\Phi^*) = \Delta^{mn}$.
\end{proof}

\begin{observation}
    The set $\cP^\varepsilon$ contains a $\varepsilon$-ball in $mn$-dimensional space.
\end{observation}

\begin{lemma}
    The set $\cS$ is convex.
\end{lemma}
\begin{proof}
Consider two k-CSPs $\Phi^{1}$ and $\Phi^{2}$ such that $C(\Phi^{1})$ and $C(\Phi^{2})$ are both valid menus. Let $\Phi' = \alpha \Phi^{1} + (1-\alpha)\Phi^{2}$. Then, our goal is to prove that $C(\Phi')$ is a valid menu. To do this, we will propose a candidate algorithm which has a menu contained within $C(\Phi')$. Let us refer to $\A_{1}$ as an algorithm with the menu $C(\Phi^{1})$ and $\A_{2}$ as an algorithm with the menu $C(\Phi^{2})$. These algorithms must exist, given our assumptions that $\Phi^{1}$ and $\Phi^{2}$ are in $\cS$. Then our new algorithm $\A'$ is as follows. It will initialize algorithms $\A_{1}$ and $\A_{2}$. Then, at each time step $t$ given a sequence of optimizer actions so far $s^{1:t}$, it will play $\alpha \A_{1}(s^{1:t}) + (1 -\alpha) \A_{2}(s^{1:t})$. We claim that $\M(\A') \subseteq C(\Phi')$, and therefore that $C(\Phi')$ is a menu. 
Let us assume for contradiction that this is not the case. Then, there is a sequence $s$ that the optimizer can play such that the resulting CSP is not in $C(\Phi')$. Note that $C(\Phi')$ is the set of all CSPs $x$ such that, for all $i$, $u_{O,i}(\Phi'_i) \geq u_{O,i}(x)$. Thus, there is a sequence that the optimizer can play against $\A'$ such that in the resulting CSP $x$, there is some $i$ s.t. $u_{O,i}(\Phi'_i) < u_{O,i}(x)$. So we have

\begin{align*}
u_{O,i}(\Phi'_i) < u_{O,i}(\A'(s)) &
\\ & \implies u_{O,i}(\alpha \Phi^{1}_{i} + (1 - \alpha) \Phi^{2}_{i}) < u_{O,i}(\A'(s)) \\
& \implies u_{O,i}(\alpha \Phi^{1}_{i} + (1 - \alpha) \Phi^{2}_i) < u_{O,i}(\alpha \A_{1}(s) + (1 - \alpha)\A_{2}(s)) \tag{By the definition of $\A'$} \\
& \implies \alpha u_{O,i}(\Phi^{1}_i) + (1 - \alpha) u_{O,i}(\Phi^{2}_i) < \alpha u_{O,i}(\A_{1}(s)) + (1 - \alpha)u_{O,i}(\A_{2}(s)) \tag{By the linearity of $u_{O,i}$} \\
& \implies \alpha (u_{O,i}(\Phi^{1}_i) - u_{O,i}(\A_{1}(s)))  <  (1 - \alpha)(u_{O,i}(\A_{2}(s)) - u_{O,i}(\Phi^{2}_i))  \\
& \implies \alpha (0)  <  (1 - \alpha)(u_{O,i}(\A_{2}(s)) - u_{O,i}(\Phi^{2}_i)) \tag{By the definition of $\A_{1}$} \\
& \implies \alpha (0)  <  (1 - \alpha)(0) \tag{By the definition of $\A_{2}$} \\
\end{align*}

This derives a contradiction. Therefore the menu of $\A'$ is contained within $C(\Phi')$. By the upward-closedness of menus, $C(\Phi')$ is also a valid menu, and therefore $\Phi' \in S$.
\end{proof}

\begin{lemma}
    The set $\cR$ is convex.
\end{lemma}
\begin{proof}
    Consider two k-CSPs $\Phi^{1}$ and $\Phi^{2}$ such that $\Phi^{1}$ and $\Phi^{2}$ are in $\cR$. Then, our goal is to prove that $\Phi' = \alpha \Phi^{1} + (1-\alpha)\Phi^{2}$ is in $\cR$. Assume for contradiction that this is not the case. Then, there is some $(i,j)$ pair such that 
    
\begin{align*}
 u_{O,i}(\Phi'_{i}) < u_{O,i}(\Phi'_{j}) \\
& \implies u_{O,i}(\alpha \Phi^{1}_i + (1 - \alpha) \Phi^{2}_i) < u_{O,i}(\alpha \Phi^{1}_j + (1 - \alpha) \Phi^{2}_j) \\
& \implies \alpha u_{O,i}(\Phi^{1}_i) + (1 - \alpha) u_{O,i}(\Phi^{2}_i) < \alpha u_{O,i}(\Phi^{1}_j) + (1 - \alpha) u_{O,i}(\Phi^{2}_j) \tag{By the linearity of $u_{O,i}$} \\
& \implies \alpha (u_{O,i}(\Phi^{1}_i) -  u_{O,i}(\Phi^{1}_j)) < (1 - \alpha) (u_{O,i}(\Phi^{2}_j)  - u_{O,i}(\Phi^{2}_i)) \\
& \implies \alpha (0) < (1 - \alpha) (0) \tag{By the fact that $\Phi^{1}$ and $\Phi^{2}$ are in $\cR$} \\
\end{align*}

This derives a contradiction, and therefore $\Phi'$ is also in $\cR$.

\end{proof}
\subsection{Main Results}

\begin{theorem}[~\cite{mannor2009approachability}]
\label{thm:tsitsiklis}
    There is an algorithm with running time $\min \left\{ \text{Poly}(\frac{mn}{\varepsilon}) \cdot 2^{\text{Poly}(k)}, \text{Poly}(\frac{k}{\varepsilon}) \cdot 2^{\text{Poly} (mn)}\right\}$ which, given a polytope $D$ in $mn$ dimensional space, correctly outputs one of the following two results:
    \begin{itemize}
        \item $D^{\epsilon}$ is approachable
        \item $D$ is not approachable
    \end{itemize}
\end{theorem}

\begin{theorem}
\label{thm:approachability_oracle}
    There is an algorithm with running time $\min \left\{ \text{Poly}(\frac{mn}{B\varepsilon}) \cdot 2^{\text{Poly}(k)}, \text{Poly}(\frac{k}{B\varepsilon}) \cdot 2^{\text{Poly} (mn)}\right\}$ that is a $2\varepsilon$-membership oracle for the set $\cS$.
\end{theorem}

\begin{proof}
The algorithm operates as follows: given some k-CSP $\Phi$, compute the result of \ref{thm:tsitsiklis} on $C(\Phi)$ using the approximation parameter of $B \epsilon$. This will reveal either that $C(\Phi)^{B\epsilon}$ is approachable, or $C(\Phi)$ is not approachable. In the first case, our algorithm outputs that $\Phi \in \cS^{2\epsilon}$. in the second case, our algorithm outputs that $\Phi \notin \cS$.

First, we will show that if $C(\Phi)^{B\epsilon}$ is approachable, then $\Phi \in \cS^{2\epsilon}$. To see this, consider a new polytope $M$, defined as follows: 
\[ M := \{ \phi \in \Delta^{mn} | u_{O,i}(\phi) \le u_{O,i}(\Phi_i) + 2 B \epsilon, \forall i \in [k] \}\]

$C(\Phi)^{B\epsilon} \subseteq M$. Therefore, $M$ is approachable. Now, let us consider $M'$, a subset of $M$, defined as follows:
\[ M' := \{ \phi \in \Delta^{mn} | u_{O,i}(\phi) \le \min(u_{O,i}(\Phi_i) + 2B\epsilon, L+_{i}), \forall i \in [k] \}\]

Note that the only points in $M \backslash M'$ are points $\phi$ such that, for some $i$, $u_{O,i}(\phi) > L+_{i}$. It is not possible for these to be generated by any sequence against any algorithm. Therefore, as $M'$ is a subset of $M$ containing all possibly reachable CSPs in $M$, and $M$ is approachable, then $M'$ is approachable.

Now, consider the k-CSP $\Phi^{*}$ which strictly increases the utility of every agent by $2 B \epsilon$ in the following way: for every $i$, for $\Phi_{i}$, decrease the weight on the worst move pairs for agent $i$ until weight has been decreased by $2\epsilon$, and increase the weight on $L+_{i}$ by $2\epsilon$. In doing this, for every $i$, there are two possibilities:
\begin{itemize}
    \item There is at least $2\epsilon$ weight on action pairs that are not $L+_{i}$. Then, $u_{O,i}(\Phi_{i}^{*}) > u_{O,i}(\Phi_{i}) + 2B\epsilon$, where $B$ is the smallest gap between utilities in the game. 
    \item $\Phi_{i}^{*} = L+$. 
\end{itemize}

Thus, we have that for all $i$, $u_{O,i}(\Phi^{*}_{i}) \geq \min(u_{O,i}(\Phi_i) + 2B\epsilon, L+_{i})$. Therefore, $C(\Phi^{*}) \supseteq M'$, and since $M'$ is approachable, $C(\Phi^{*})$ is approachable. Therefore, $\Phi^{*} \in \cS$.

Now, note that the distance between $\Phi^{*}$ and $\Phi$ is at most $2 \epsilon$, by construction. Furthermore, recall that $\Phi^{*} \in \cS$. Therefore, $\Phi \in \cS^{2 \epsilon}$.

Finally, we must show that, if $C(\Phi)$ is not approachable, then $\Phi \notin \cS$. But this follows directly from the definition of $\cS$, so we are done.

\end{proof}

\begin{lemma}
    \label{lemma:ic_membership}
    There is a polynomial time membership oracle for the set $\cR$.
\end{lemma}

\begin{corollary}
\label{corollary:intersection_membership}
    There is an algorithm with running time $\min \left\{ \text{Poly}(\frac{mn}{\varepsilon}) \cdot 2^{\text{Poly}(k)}, \text{Poly}(\frac{k}{\varepsilon}) \cdot 2^{\text{Poly} (mn)}\right\}$ that is a $\varepsilon$-membership oracle for the (convex) set $\cR^\varepsilon \cap \cS^\varepsilon$.
\end{corollary}

\subsection{Proof of Theorem~\ref{thm:main_result_without_nr}}
\begin{proof}
    
   We employ the membership oracle in Corollary~\ref{corollary:intersection_membership} and a standard algorithm to optimize a linear function in a convex set (see~\cite{grotschel2012geometric}) to give us $x \in \cR^\varepsilon \cap \cS^\varepsilon$ such that $V_L(x) \ge \max_{y \in \cR^\varepsilon \cap \cS^\varepsilon} V_L(y) - \delta$. The running time of this algorithm is $\log{\left(\frac{1}{\delta} \right)} \cdot \min \left\{ \text{Poly}(\frac{mn}{\varepsilon}) \cdot 2^{\text{Poly}(k)}, \text{Poly}(\frac{k}{\varepsilon}) \cdot 2^{\text{Poly} (mn)}\right\}$. Since $\cP \subseteq \cR^\varepsilon \cap \cS^\varepsilon$, Lemma~\ref{lemma:wlog_polytope} implies that $V^* \le \max_{y \in \cR^\varepsilon \cap \cS^\varepsilon} V_L(y)$, implying that $V_L(x) \ge V^* -\delta$.

Since $x \in \cR^\varepsilon \cap \cS^\varepsilon$, there exist points $ r \in \cR$ and $s \in \cS$ such that $d(x,r) \le \varepsilon$ and $d(x,s) \le \varepsilon$. The triangle inequality gives $d(r,s) \le 2 \varepsilon$.
    
     Since all the payoff vectors are within the bounds $[-1,1]^{mn}$, $V_L(s) \ge V_L(x) -2\varepsilon \ge V^* - (2\varepsilon+\delta)$.
    
     Write $s  = (\phi_1, \phi_2 \cdots \phi_k)$ and $r  = (\phi'_1, \phi'_2 \cdots \phi'_k)$. Since $d(r,s) \le 2 \varepsilon$, $u_{O,i}(\phi_i) \ge u_{O,i}(\phi'_i) -  2 \varepsilon$ and $u_{O,i}(\phi_j) \le u_{O,i}(\phi'_j) +  2 \varepsilon$ for all $i,j \in [k]$. However, since $r \in \cR$, $u_{O,i}(\phi'_i) \ge u_{O,i}(\phi'_j)$, thus we get $u_{O,i}(\phi_i) \ge u_{O,i}(\phi_j) - 4 \varepsilon$ for all $i,j \in [k]$ ,i.e., the incentive compatibility constraints are approximately satisfied by the point $s$.
    
    Construct the set $\cM : = \text{Conv} \{\cC(s) \cup \{\phi_1,\phi_2 \cdots \phi_k\} \}$. First, we see that $\cM$ is a feasible menu, since $\cC(s)$ is a feasible menu (due to $s \in \cS$) and menus are upwards closed. Second, we see that $u_{O,i}(\phi_i) \ge u_{O,i}(\phi) - 4 \varepsilon$ for all $\phi \in \cM$ (using the properties of $\cC$ and the inequalities proved in the last step). If the optimizer type is willing to take a hit of up to $4 \varepsilon$ while best-responding in the menu $\cM$, the point $p_i$ picked by the $i$-th optimizer satisfies $u_L(p_i) \ge u_L(\phi_i)$ since we have just shown that $\phi_i$ is a candidate point for the $i$-th optimizer type.
    
    Thus, $V^{4 \varepsilon}_L(\cM) \ge V_L(S) \ge V^* - (2 \varepsilon + \delta)$, completing the proof of Theorem~\ref{thm:main_result_without_nr}.

\end{proof}
